# Supplementary material for: PyTorch Connectomics: A Scalable and Flexible Segmentation Framework for EM Connectomics
Source: arXiv:2112.05754 source file (2021-12-10)
Supplement: Supplementary file 1 [file appendix.tex]

% reset Figure number: e.g., Figure B.1.

\setcounter{figure}{0} 
\setcounter{table}{0} 

\appendix

\section{Data Augmentation Details}

\section{Post-processing}
